# Supplementary material for: Recover Fine-Grained Spatial Data from Coarse Aggregation
Source: arXiv:1803.00192 source file (2018-03-01)
Supplement: Supplementary file 1 [file appendix.tex]

\appendices

\section{Proofs of Sec.~\ref{sec:analysis}}
